# Supplementary material for: Resistive switching acceleration induced by thermal confinement
Source: arXiv:2402.07603 source file (2024-02-12)
Supplement: Supplementary file 1 [file Supporting_Information.pdf]

# Supporting Information: Resistive Switching Acceleration Induced by Thermal Confinement

Alexandros Sarantopoulos<sup>1\*</sup>, Kristof Lange<sup>2</sup> Francisco Rivadulla<sup>3</sup> Stephan Menzel<sup>2</sup> and Regina Dittmann<sup>1\*</sup>

<sup>1</sup>Peter Gruenberg Institute (PGI-7), Forschungszentrum Juelich GmbH and JARA-FIT, 52425 Juelich, Germany

<sup>2</sup>IWE2, RWTH Aachen University, Aachen 52074, Germany

<sup>3</sup>Centro de Investigación en Química Biológica y Materiales Moleculares (CIQUS), Universidad de Santiago de Compostela, 15782 Santiago de Compostela, Spain

## 01. Interlayer Characterization

We have measured the electrical resistivity of the TaO<sub>x</sub> layers that have been used as heat-blocking layers, in a van der Pauw configuration, and estimated their electrical resistivity/conductivity. The results are presented in Supporting Figure 1, showing ohmic behaviour for both samples.

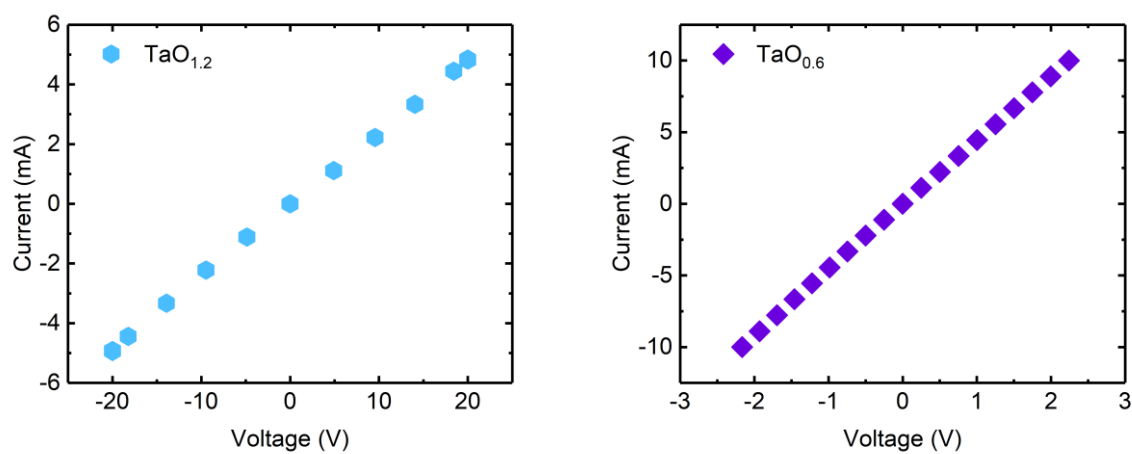

*Supporting Figure 1: Electrical characterization of the TaO<sub>x</sub> layers in a van der Pauw configuration, from which the electrical conductivity values were estimated. The behaviour of the TaO<sub>1.2</sub> sample, slightly deviates from ohmic behaviour, which is attributed to the elevated contact resistance between the sample and the aluminium wires. The estimated value of resistivity is  $7.6 \times 10^{-3}$  Ohm cm. The TaO<sub>0.6</sub> sample exhibits clearly ohmic behaviour, yielding a value of resistivity of  $2.67 \times 10^{-4}$  Ohm cm.*

To make sure the interlayers used as heat-blocking layers in our study, don't present resistive switching behaviour, we have fabricated devices with the stack Pt/HfO<sub>2</sub>/Pt on Si/SiO<sub>2</sub> substrates and measured the I-V and R-V response in the same range of voltages that were used to measure the actual STO-based devices presented in the main manuscript (see Supporting Figure 2).

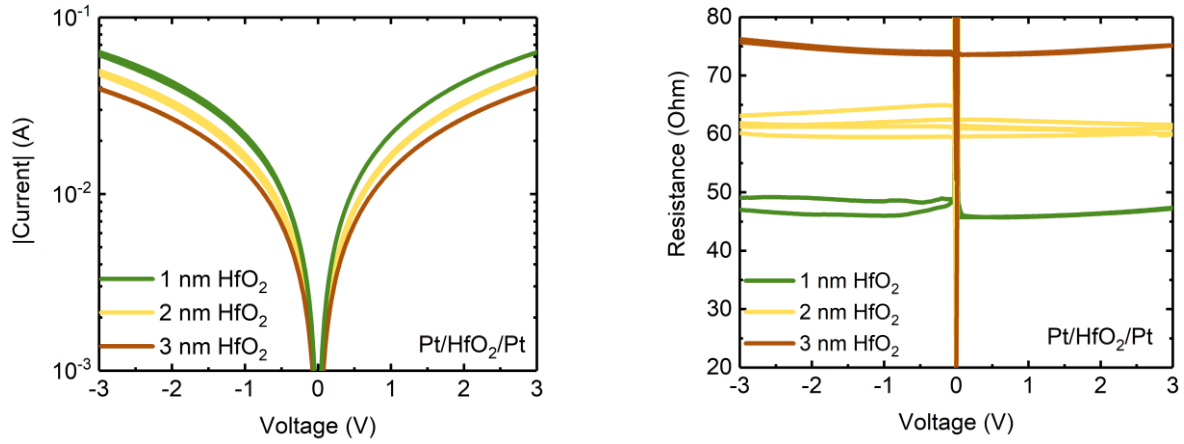

Supporting Figure 2: HfO<sub>2</sub> interlayer electrical characterization in the stack Pt/HfO<sub>2</sub>/Pt, where no resistive switching behavior is observed. The voltages applied here are the same as the ones used for the resistive switching characterization of the STO/Pt/HfO<sub>2</sub>/Pt devices. Left graph represents the I-V sweep, and the right graph the R-V sweep of the same device.

## 02. Forming and DC-switching voltage of the full devices Nb:STO/STO/Pt/interlayer/Pt.

Introducing the heat-blocking layers has a certain impact on the electrical properties of the devices, since they introduce an increased series resistance to the stack, compared to the reference STO/Pt devices. The forming and DC-switching voltage for all the devices are exhibited in Supporting Figure 3. There are two different reference samples, one labelled as STO/Pt and the second one labelled as “0 nm” in the HfO<sub>2</sub> thickness scale. Each reference sample is a 5x5mm part of a larger 10x10 mm STO thin film, to ensure that the differences observed are only due to the thermal blocking layer and not any potential differences in the STO thin film.

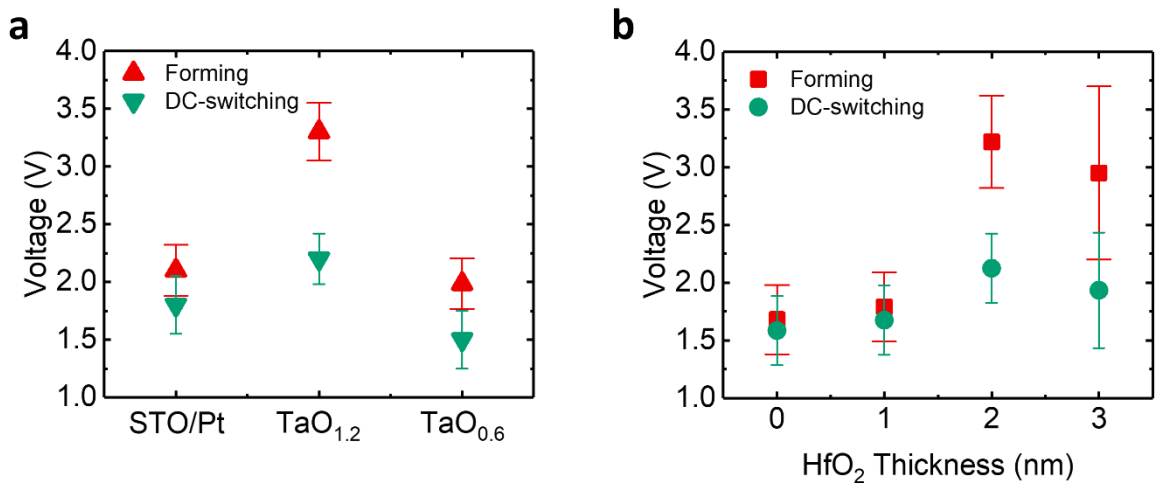

Supporting Figure 3: Forming and DC-switching voltage for the full devices using TaO<sub>x</sub> interlayers (a) and HfO<sub>2</sub> interlayers (b). The reference samples Nb:STO/STO/Pt are denominated as “STO/Pt” in the TaO<sub>x</sub> control group, and “0 nm” in the HfO<sub>2</sub> control group, respectively.

### 03. Thermal conductivity measurements using frequency domain thermoreflectance (FDTR)

The fittings were done using Matlab software. The materials' parameters used for the fittings are listed in **Supporting Table 1**. The transducer layer (Au) and the Pt layer were considered as one material with adjusted combined electrical and thermal conductivity. The interlayers were treated as an increased thermal resistance embedded inside the Pt layers, as described in the main text. The values of the thermal resistance were obtained by the inversed thermal boundary conductance (TBC) extracted by the values of the FDTR fittings. The thickness of the materials was adjusted when the layers were of different thickness in **Supporting Table 1**. The fittings for the different samples are shown in figures **Supporting Figure 4 – 7**.

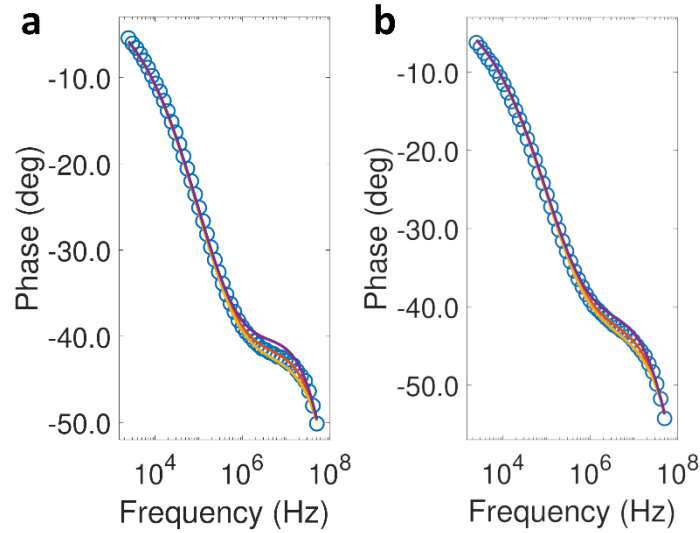

Supporting Figure 4: FDTR fittings for the STO/Pt interface for two different thicknesses of Pt: (a) 10 nm and (b) 20 nm.

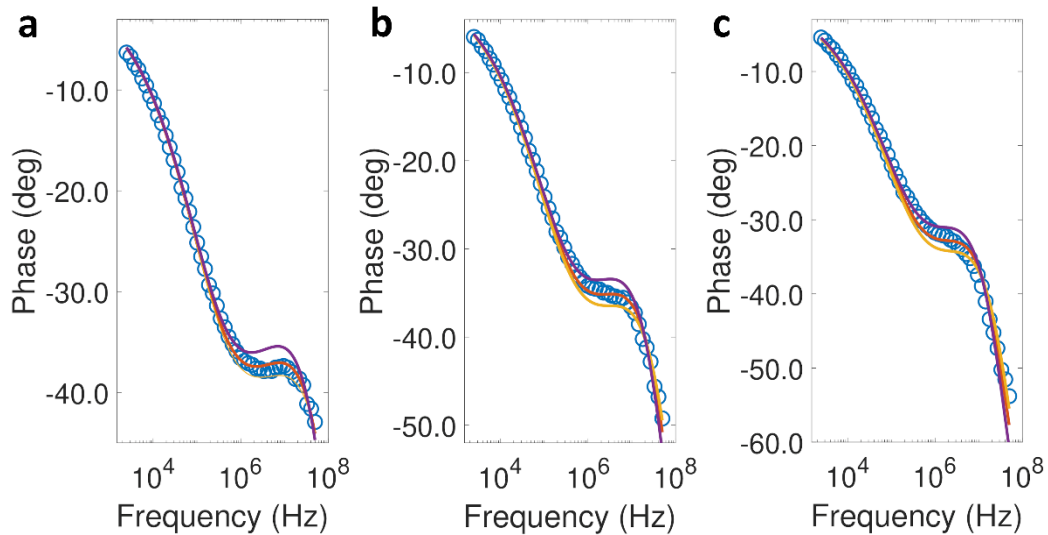

Supporting Figure 5: FDTR fittings for the  $\text{TaO}_{1.2}$  interlayers of three different thicknesses: (a) 10 nm, (b) 20 nm, and (c) 40 nm.

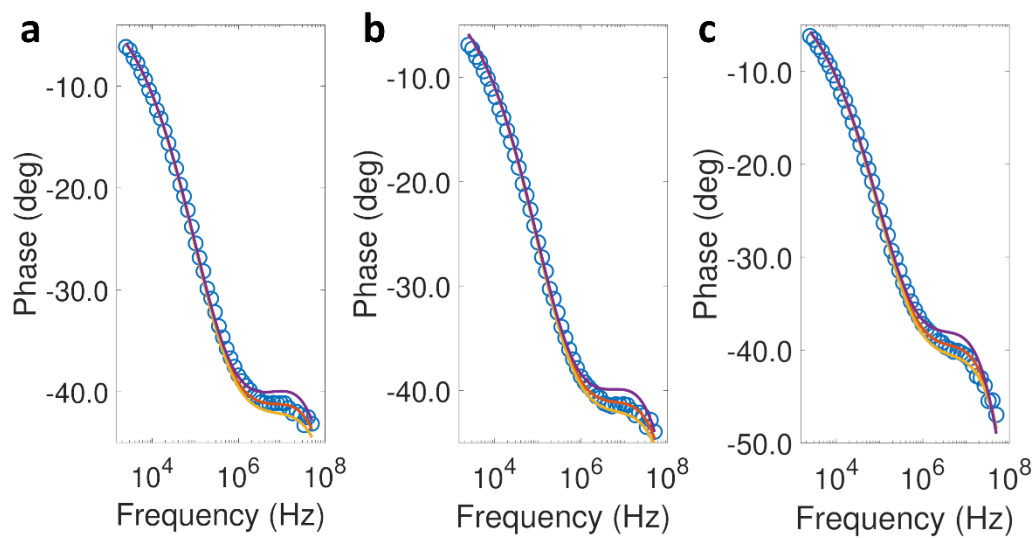

Supporting Figure 6: FDTR fittings for the  $\text{TaO}_{0.6}$  interlayers of three different thicknesses: (a) 10 nm, (b) 20 nm, and (c) 40 nm.

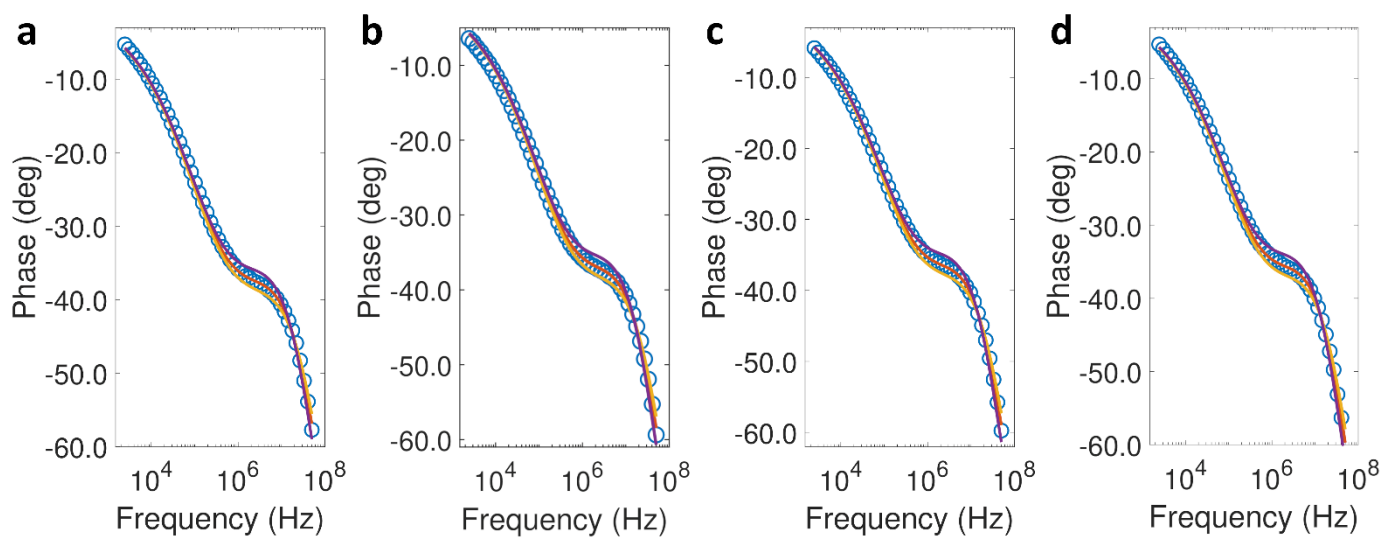

Supporting Figure 7: FDTR fittings for the  $\text{HfO}_2$  interlayers of four different thicknesses: (a) 1 nm, (b) 2 nm, (c) 3 nm, and (d) 4 nm.

**Supporting Table 1:** FDTR fittings materials' parameters.

| Property<br>Material          | C<br>(J/m <sup>3</sup> K) | κ<br>(W/m K) | Thickness<br>(m)         | TBC<br>(W/m <sup>2</sup> K) | TBR<br>(m <sup>2</sup> K/W) |
|-------------------------------|---------------------------|--------------|--------------------------|-----------------------------|-----------------------------|
| Au/Pt                         | $2.4 \cdot 10^6$          | 50           | $50 - 100 \cdot 10^{-9}$ |                             |                             |
| STO                           | $2.72 \cdot 10^6$         | 8            | $500 \cdot 10^{-6}$      |                             |                             |
| STO/Pt                        |                           |              | $10 \cdot 10^{-9}$       | $1.2 \cdot 10^8$            | 4.8E-9                      |
| STO/Pt                        |                           |              | $20 \cdot 10^{-9}$       | $1.2 \cdot 10^8$            | 4.8E-9                      |
| STO/Pt/TaO <sub>1.2</sub> /Pt |                           |              | $10 \cdot 10^{-9}$       | $7.06 \cdot 10^7$           | 14.2E-9                     |
| STO/Pt/TaO <sub>1.2</sub> /Pt |                           |              | $20 \cdot 10^{-9}$       | $4.60 \cdot 10^7$           | 21.7E-9                     |
| STO/Pt/TaO <sub>1.2</sub> /Pt |                           |              | $40 \cdot 10^{-9}$       | $3.2 \cdot 10^7$            | 31.1E-9                     |
| STO/Pt/TaO <sub>0.6</sub> /Pt |                           |              | $10 \cdot 10^{-9}$       | $1.51 \cdot 10^8$           | 6.6e-9                      |
| STO/Pt/TaO <sub>0.6</sub> /Pt |                           |              | $20 \cdot 10^{-9}$       | $1.09 \cdot 10^8$           | 9.2e-9                      |
| STO/Pt/TaO <sub>0.6</sub> /Pt |                           |              | $40 \cdot 10^{-9}$       | $8.62 \cdot 10^7$           | 11.6e-9                     |
| STO/Pt/HfO <sub>2</sub> /Pt   |                           |              | $1 \cdot 10^{-9}$        | $5.31 \cdot 10^7$           | 18.8E-8                     |
| STO/Pt/HfO <sub>2</sub> /Pt   |                           |              | $2 \cdot 10^{-9}$        | $4.88 \cdot 10^7$           | 20.5E-8                     |
| STO/Pt/HfO <sub>2</sub> /Pt   |                           |              | $3 \cdot 10^{-9}$        | $4.54 \cdot 10^7$           | 22.0E-8                     |
| STO/Pt/HfO <sub>2</sub> /Pt   |                           |              | $4 \cdot 10^{-9}$        | $4.10 \cdot 10^7$           | 24.3E-8                     |

#### 04. FEM simulation of temperature distribution during switching

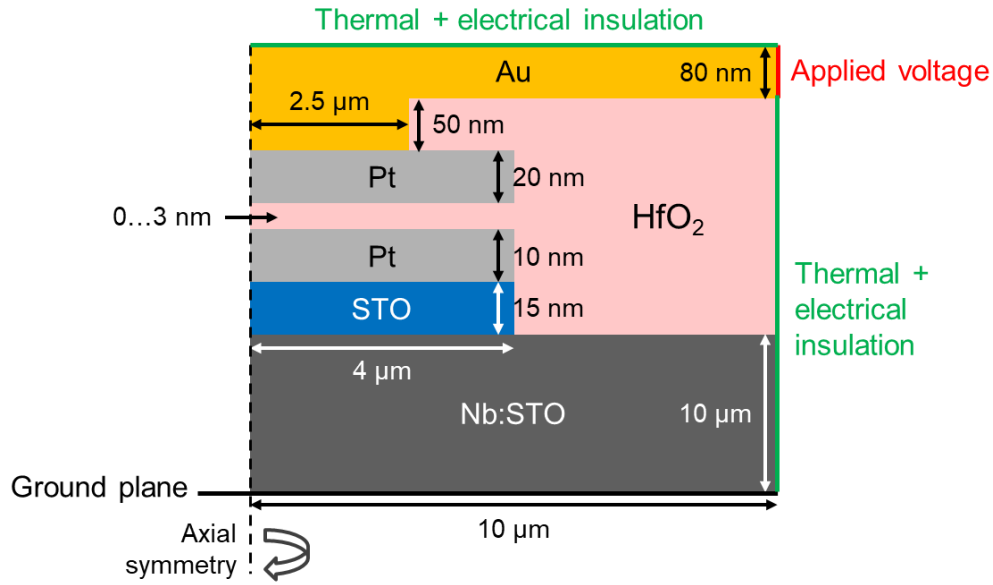

Supporting Figure 8: Simulated device structure, shown schematically (not to scale).

In order to study the effect of an  $\text{HfO}_2$  interlayer with a thickness of 1 nm, 2 nm, or 3 nm within the Pt layer of an Au/Pt/STO/Nb:STO stack, FEM simulations have been performed using the device structure shown in Supporting Figure 1. The bottom edge of the Nb:STO layer is fixed at  $V = 0$  V and a voltage is applied to the outer edge of the Au layer. At both interfaces, the temperature is constant with  $T = T_{\text{amb}} = 293.15$  K, while every other exterior surface is thermally insulated. **Supporting Table 2** shows the material parameters as used in the simulations. The device radius  $r_{\text{device}} = 4 \mu\text{m}$  and channel radius  $r_{\text{channel}} = 2.5 \mu\text{m}$  are derived from a device area of  $48 \mu\text{m}^2$  and an opening area of  $20 \mu\text{m}^2$  in fabricated devices.

**Supporting Table 2:** Material parameters as used in the simulation.

| Material                  | $\sigma$ [S/m]    | $\kappa$ [W/(m·K)] | $C_p$ [J/(kg·K)] | $\rho$ [kg/m <sup>3</sup> ] |
|---------------------------|-------------------|--------------------|------------------|-----------------------------|
| Au                        | $3.33 \cdot 10^6$ | 60                 | 129              | $19.3 \cdot 10^3$           |
| Pt                        | $1.66 \cdot 10^6$ | 44.5               | 126              | $22.03 \cdot 10^3$          |
| STO                       | User defined      | 5.4                | 532              | $4.81 \cdot 10^3$           |
| Nb:STO                    | $1 \cdot 10^6$    | 8.7                | 532              | $4.81 \cdot 10^3$           |
| $\text{HfO}_2$ interlayer | $1.66 \cdot 10^6$ | 0.53               | 120              | $6.99 \cdot 10^3$           |
| outer $\text{HfO}_2$      | -                 | 1                  | 120              | $6.99 \cdot 10^3$           |

The equation system that is solved during the simulations mainly comprises two equations, one to calculate the electric potential and one to calculate the temperature. A stationary equation for current conservation of the form

$$\nabla \cdot J = \nabla(\sigma E) = -\nabla(\sigma \nabla V) = 0 \quad (1)$$

is used for the electric potential  $V$  and current density  $J$ , where  $\sigma$  denotes the electrical conductivity and  $E$  the electric field. The temperature  $T$  is given by the time-dependent heat transfer equation

$$\rho C_p \frac{\partial T}{\partial t} - \nabla(\kappa \nabla T) = Q_{\text{Joule}} = J \cdot E = \frac{J^2}{\sigma} \quad (2)$$

with the density  $\rho$ , the heat capacity  $C_p$ , and the thermal conductivity  $\kappa$ .  $Q_{\text{Joule}}$  is the heat energy generated by Joule heating. Equation (2) is solved everywhere, whereas equation (1) is solved everywhere except for the outer  $\text{HfO}_2$  domain. As initial conditions,  $V_{\text{init}} = 10^{-9} \text{ V}$  and  $T_{\text{init}} = T_{\text{amb}}$  are used.

The applied voltage is taken from a measured  $I$ - $V$  sweep during switching, and the electrical conductivity of the STO layer  $\sigma_{\text{STO}}$  is fitted to match the corresponding current. To reach reasonable temperatures and to be able to fit measured switching kinetics, the conduction is confined to a filament with radius  $r_{\text{filament}} = 200 \text{ nm}$ . Within this filament,  $\sigma_{\text{STO}}$  can thus be calculated as

$$\sigma_{\text{STO, filament}} = \left| \frac{I_{\text{input}}}{V_{\text{input}}} \right| \cdot \frac{h_{\text{STO}}}{\pi r_{\text{filament}}^2} \quad (3)$$

with the measured current  $I_{\text{input}}$  and voltage  $V_{\text{input}}$ , and the thickness of the STO layer  $h_{\text{STO}}$ . In the bulk oxide outside of the filament, the conductivity is lowered by a factor of  $10^{-9}$ , i.e.  $\sigma_{\text{STO, bulk}} = 10^{-9} \cdot \sigma_{\text{STO, filament}}$ , so that the current through the bulk is negligible. With the assumption of  $\sigma_{\text{HfO}_2, \text{interlayer}} = \sigma_{\text{Pt}}$  to focus on thermal effects, there is no significant voltage drop across the interlayer.

When the filament radius is changed, then the calculated temperature and heating efficiency also change, although the trend among the different samples stays the same, as depicted in **Supporting Figure 9** for filament radii of 300 nm (a, b) and 150 nm (c, d).

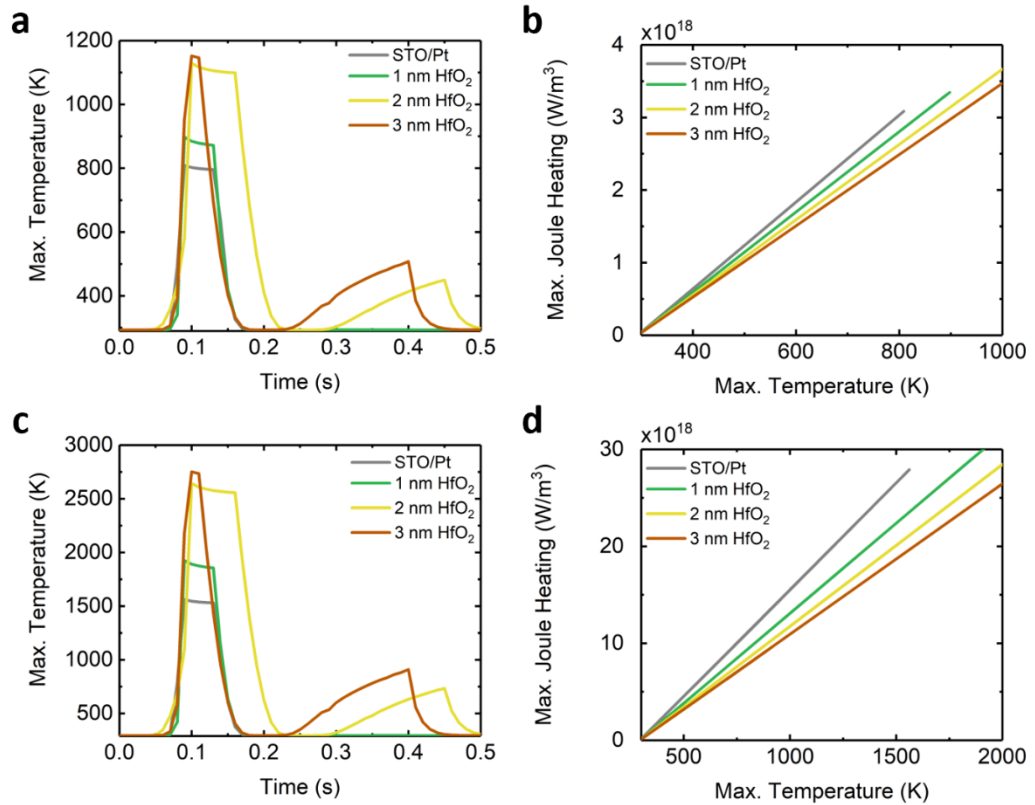

Supporting Figure 9: Local maximum temperature and heating efficiency for the reference STO/Pt devices and the devices with  $\text{HfO}_2$  interlayer (1-3 nm), for two different filament radii, (a – b): 300 nm and (c – d): 150 nm.
